# Supplementary material for: Topological electronic structure of YbMg$_2$Bi$_2$ and CaMg$_2$Bi$_2$
Source: arXiv:2205.03678 source file (2022-05-07)
Supplement: Supplementary file 1 [file Supporting_Information.pdf]

# Topological electronic structure of $YbMg_2Bi_2$ and $CaMg_2Bi_2$

Asish K. Kundu[1, *], Tufan Roy[2], Santanu Pakhira[3], Ze-Bin Wu[1], Masahito Tsujikawa[2, 4], Masafumi Shirai[2, 4, 5], D. C. Johnston[3, 6], Abhay N. Pasupathy[1, 7], and Tonica Valla[1]

[1]Condensed Matter Physics and Materials Science Division, Brookhaven National Laboratory, Upton, New York 11973, USA
[2]Research Institute of Electrical Communication, Tohoku University, Sendai 980-8577, Japan

[3]Ames Laboratory, Iowa State University, Ames, Iowa 50011, USA

[4]Center for Spintronics Research Network, Tohoku University, Sendai 980-8577, Japan

[5]Center for Science and Innovation in Spintronics, Core Research Cluster, Tohoku University, Sendai 980-8577, Japan

[6]Department of Physics and Astronomy, Iowa State University, Ames, Iowa 50011, USA

[7]Department of Physics, Columbia University, New York, NY, 10027, USA

* akundu@bnl.gov

## Electronic structure of $YbMg_2Bi_2$ for different *U* values

Figures S1(a) and S1(b) show the bulk electronic structure of $YbMg_2Bi_2$ for $U$ = 6 and 8 eV, respectively. As $U$ increases, only the Yb-4*f* states (flat-bands) move to the higher binding energy side without affecting the low-energy electronic structure.

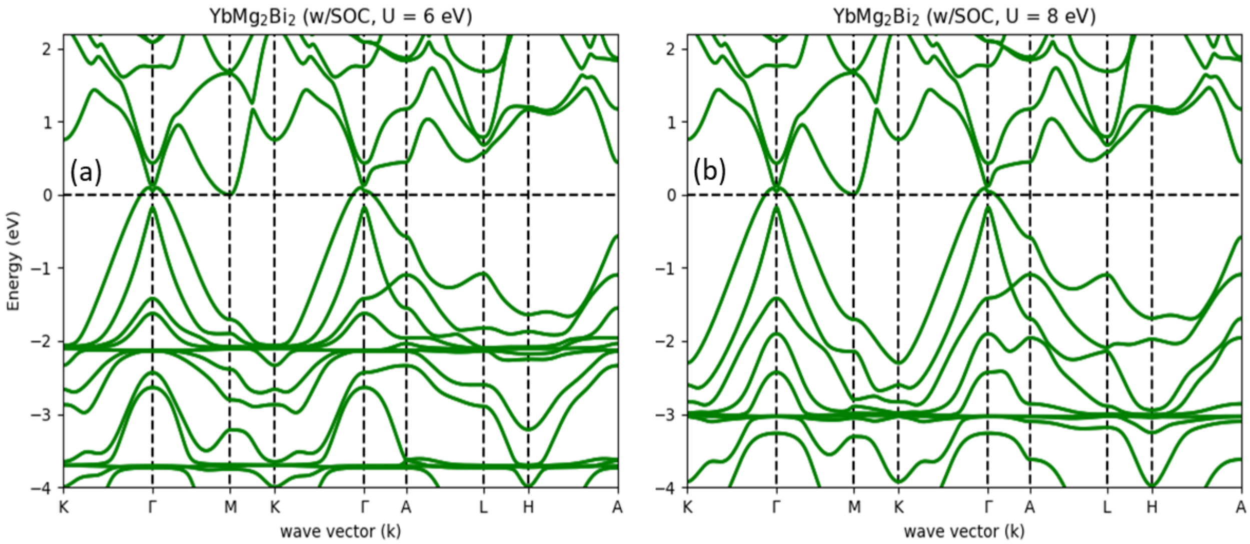


Figure S1. Bulk electronic structure of $YbMg_2Bi_2$ for different values of $U$ and including SOC. (a) and (b) $U$ = 6 eV and $U$ = 8 eV, respectively.

## Electronic structure of $YbMg_2Bi_2$ measured using He II photons (40.8 eV)

In Fig. S2, the valence-band electronic structure of $YbMg_2Bi_2$ is shown. Two intense flat-bands are seen in the spectra [Fig. (a)], originating from the Yb-4*f* levels. Dispersive bands are also seen but they are very faint for the photon energy used due to their low photoelectron cross-section. In Fig. S2(b), two hole-like bands can be seen, similar to those observed in Fig. 4(c) in the main text.

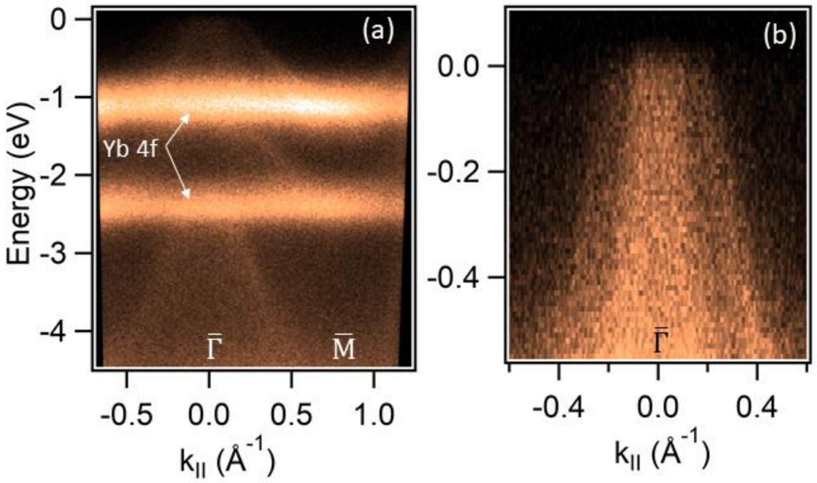


Figure S2. Valence-band electronic structure of $YbMg_2Bi_2$ using He II photons (40.8 eV). (a) ARPES spectra of $YbMg_2Bi_2$ along $\bar{\Gamma}$—$\bar{M}$ from the second SBZ. (b) Zoomed view close to the Fermi energy.

## Comparison of the dispersion of electronic states between 1st and 2nd SBZ: $YbMg_2Bi_2$

ARPES spectra close to the Fermi level ($E_F$) around the $\bar{\Gamma}$ point from the first and second surface Brillouin zones (SBZ) are shown in Fig. S3(a) and S3(b), respectively. Three linearly-dispersive bands in Fig. S3(a) are marked by the numbers 1, 2, and 3. Between the first and second zone, a visible change of the Fermi wave vector ($k_F$) of these bands can be seen. For better realization of this change, momentum dispersion curves (MDC) are

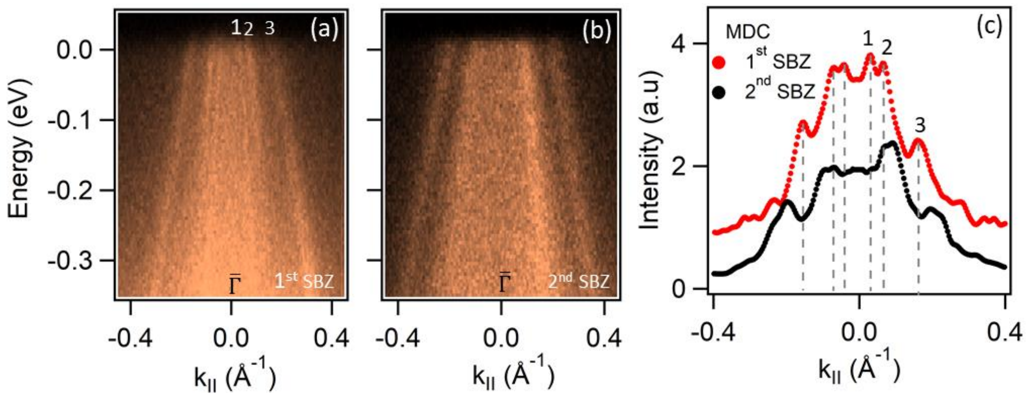

Figure S3. ARPES spectra and MDC curves of $YbMg_2Bi_2$. (a) and (b) ARPES spectra close to the Fermi level between the first and second SBZ. (c) MDC curves around $E_F$ plotted together for first and second zone around $E_F$.

shown in Fig. S3(c). In the first SBZ, at the position of peaks 1 and 3, we see a clear dip in the second SBZ. This strongly suggests that they are originating from the bulk bands. Apparently, the position of peak 2 seems constant between first and second zone, suggesting its surface origin. Considering the bulk electronic structure, it is also expected that there should be only two bulk bands that might cross $E_F$, consistent with our observation.

## Electronic structure of $YbMg_2Bi_2$ after 12 min of potassium deposition

Figure S4 shows the valence-band electronic structure of $YbMg_2Bi_2$ after 12 min potassium deposition on the surface of the as-cleaved sample. In Fig. S4(a), a small photoemission intensity forming a nearly V-shape, just below the $E_F$ can be seen. By superimposing bulk electronic bands on the spectra [Fig. S4(b)], it seems to appear from the conduction band. It is also possible that the intensity originates from a mixture of a topological surface state and conduction band electron states.

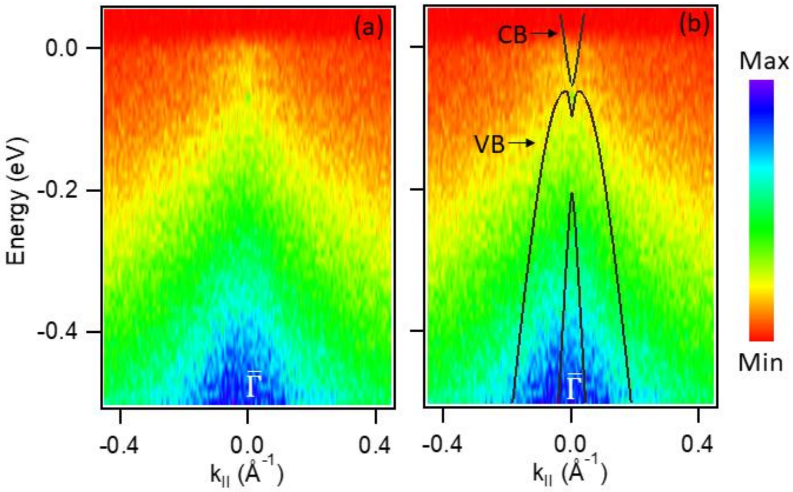


Figure S4. (a) ARPES spectrum around the $\bar{\Gamma}$ point for the 12 min potassium-deposited sample. (b) Bulk bands (black-lines) from first-principles calculations are superimposed on the spectra. A rigid energy shift has been applied on the theoretical bands as discussed in the main text. Valence and conduction bands are marked by VB and CB, respectively.

## Energy shift of the Yb-4*f* and Bi-5*d* states of $YbMg_2Bi_2$ upon potassium deposition

In Fig. S5, the evolution of the core levels and of the valence-band electronic structure upon potassium deposition are shown for $YbMg_2Bi_2$. Upon potassium deposition, an energy shift of the Bi-5*d* core-levels and Yb-4*f* valence states are seen in Fig. S5(a). In Fig. S5(b), deposition time vs. the relative energy shifts of the Bi-5*d* and Yb-4*f* levels are shown. A very similar energy shift of the core (Bi 5*d*) and the valence levels (Yb-4*f*) is observed. This suggest a nearly rigid band shift scenario upon surface potassium deposition. There is no change in the energy position of the potassium core-level (K 3*p*), indicating it is just adsorbed on the surface of the sample.

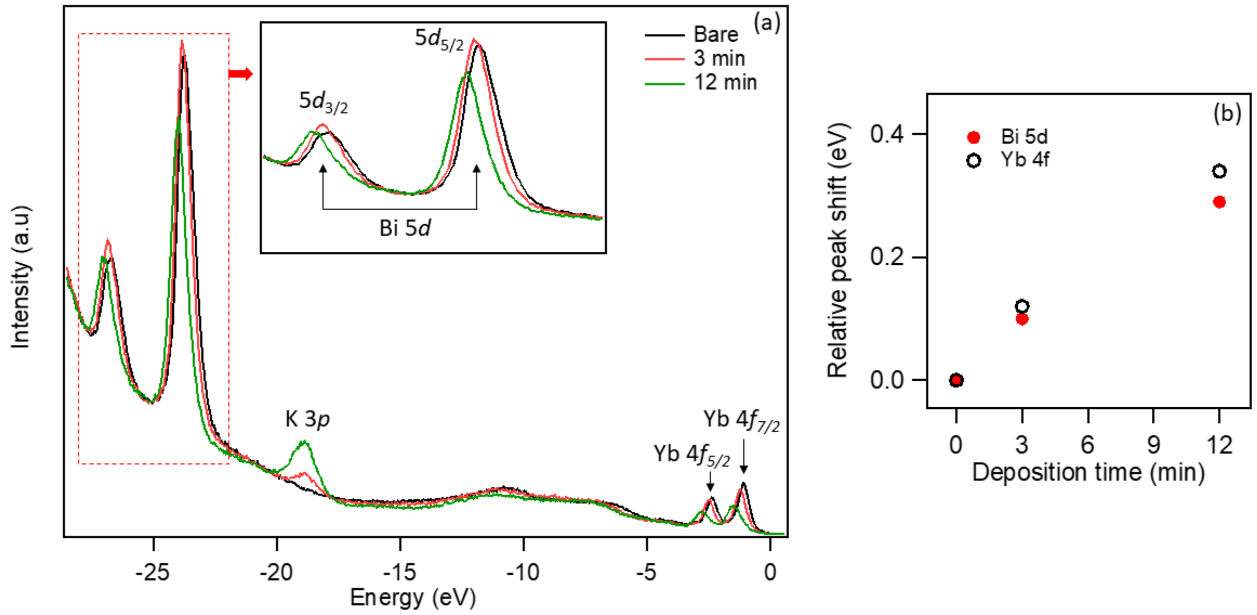


Figure S5. Evolution of the core levels and valence band electronic structure of $YbMg_2Bi_2$ upon potassium deposition. (a) The spectra taken using He II photons (40.8 eV) for the as-cleaved (bare) and 3 min and 12 min potassium-deposited samples. Inset: The zoomed view of the spectra within the dotted rectangular region. (b) The relative energy shift (shift w.r.t. as-cleaved sample) of the Yb-4*f* and Bi-5*d* levels versus potassium deposition time.

## Atomic force microscopy (AFM) on cleaved $YbMg_2Bi_2$

In Fig. S6, the AFM topography images at different positions of the cleaved $YbMg_2Bi_2$ sample are presented. The inset of Fig. S6(a) shows the optical image of the cleaved surface with the AFM cantilever tip hanging on top of it, where major and large steps are resolved. AFM images were taken at different regions (I, II, and III) of the sample as indicated in the inset, are shown in Fig. S6(a)–S6(c). The sample was cleaved right before the AFM measurement to minimize exposure to the air. However, the surface is not chemically inert to avoid the reaction with ambient. As it can be seen from the AFM images, the surface contains many islands/blobs, which were probably caused by contamination from air exposure. Figure S6(d) shows the line-cut profile as indicated in the inset of Fig. S6(b). This emphasizes the importance of *in-situ* measurement by ARPES under ultra-high vacuum.

Regardless of the surface contaminations, different surface steps are resolved in AFM. In Fig. S6(a), various small steps coexist. The step heights range from ~ 2 to ~ 4 nm, as shown in the line-cut profile in Fig. S6(e). In Fig. S6(c), a large step with height of ~100 nm is resolved. As the probing scale of the AFM is within a few micrometers, multiple surface steps/terminations will likely appear within the probing area of light beams (beam size ~ 1 mm) in our ARPES measurements.

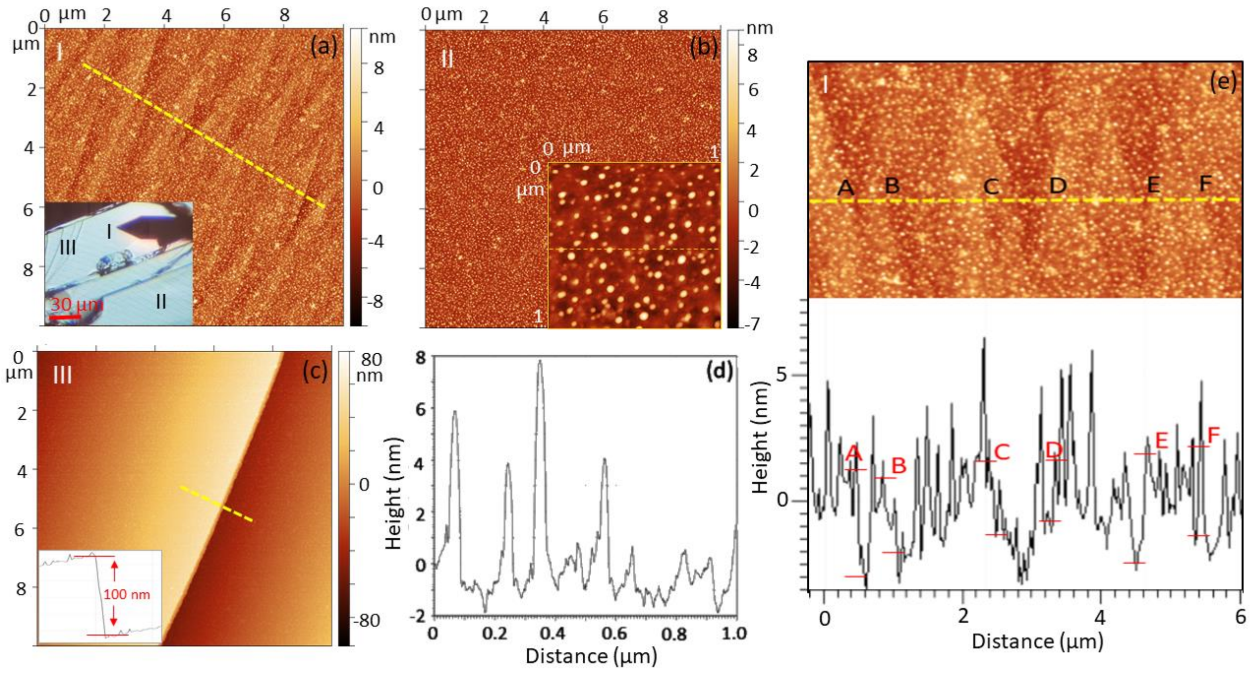


Figure S6. AFM characterization of $YbMg_2Bi_2$. (a)–(c) AFM images at different positions on sample, I, II, and III, respectively, as marked in the inset of (a). The inset of (a) is an optical image of the freshly-cleaved surface before AFM measurements. The inset of (b) is a zoomed view of (b). (d) Line profile along the dashed line shown in the inset of (b). (e) Zoomed view of (a) and the line profile along the dashed line.

## <u>Atomic force microscopy on cleaved $CaMg_2Bi_2$</u>

In Fig. S7, the AFM topography and the height-profile of the cleaved surface of $CaMg_2Bi_2$ are shown. Similar AFM topographies are resolved as on cleaved $YbMg_2Bi_2$. Both the blob-like features and the surface steps are seen in Fig. S7(a). To get better estimation of the step heights, the high-intensity blobs were artificially removed and filled those positions with the average intensity, shown in Fig. S6 (b). The step heights, ranging from ~ 2 to ~ 4 nm, are shown in Fig. S7(c). This suggests multiple surface terminations can be present within the probed area by ARPES.

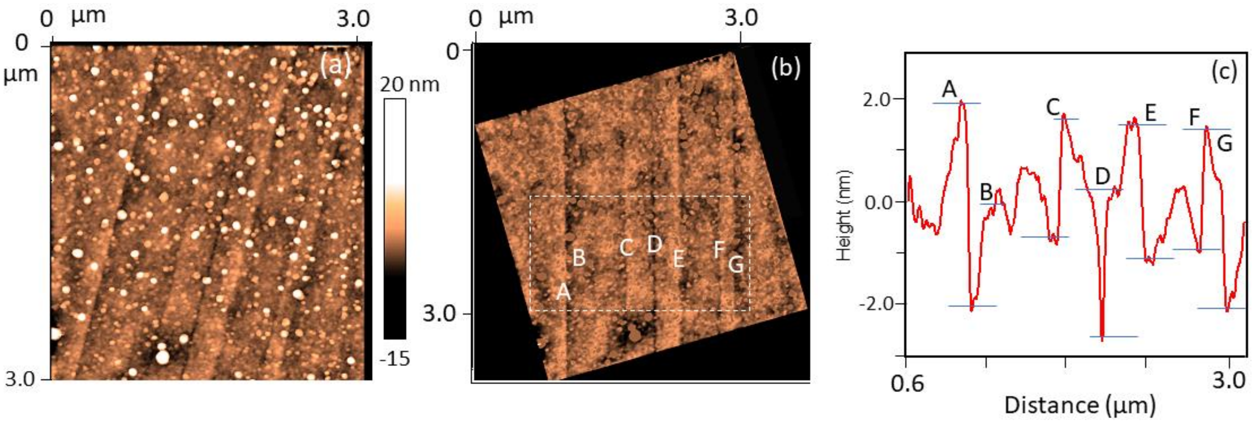


Figure S7. AFM characterization of $CaMg_2Bi_2$. (a) AFM topography of the cleaved $CaMg_2Bi_2$. (b) High-intensity blobs are artificially removed from (a) and rotated the image by 16 degree counter-clock-wise. Step edges are marked with A through G. (c) Integrated intensity profile within the dashed-rectangle as shown in (b). Step heights corresponding to the various steps are marked by horizontal lines (blue color).
